# Supplementary material for: Fairness Implications of Encoding Protected Categorical Attributes
Source: arXiv:2201.11358 source file (2023-05-05)
Supplement: Supplementary file 1 [file oldappendix.tex]

\section*{Appendix}\label{sec:appendix}
\subsection*{Data: Law School Admission Council}\label{data:lawschool}

The Law School Admission Council dataset \cite{KusnerLRS2017_CounterfactualFairness}, is based on a survey conducted by the Law School Admission Council across 163 law schools in the United States \cite{Wightman1998_LawDataSource}. It covers 21,790 students and includes their race, gender, undergraduate grade-point average (UGPA), law-school entrance exam scores (LSAT), and their first-year law-school average grade normalized by region (ZFYA). The goal is to predict ZFYA for future success in law school. The protected attributes are race and sex. Race has 8 unique groups and Sex just two. In the intersectional fairness problem, derived from feature engineering \textit{RaceSex}, the cardinality of the new categorical variable has 16 distinct values. The data is split into a 50/50 train/test split, maintaining the ratio of each category between train and test set.

\begin{figure}[ht]
\centering
\begin{subfigure}{.5\textwidth}
  \centering
  \includegraphics[width=1.2\linewidth]{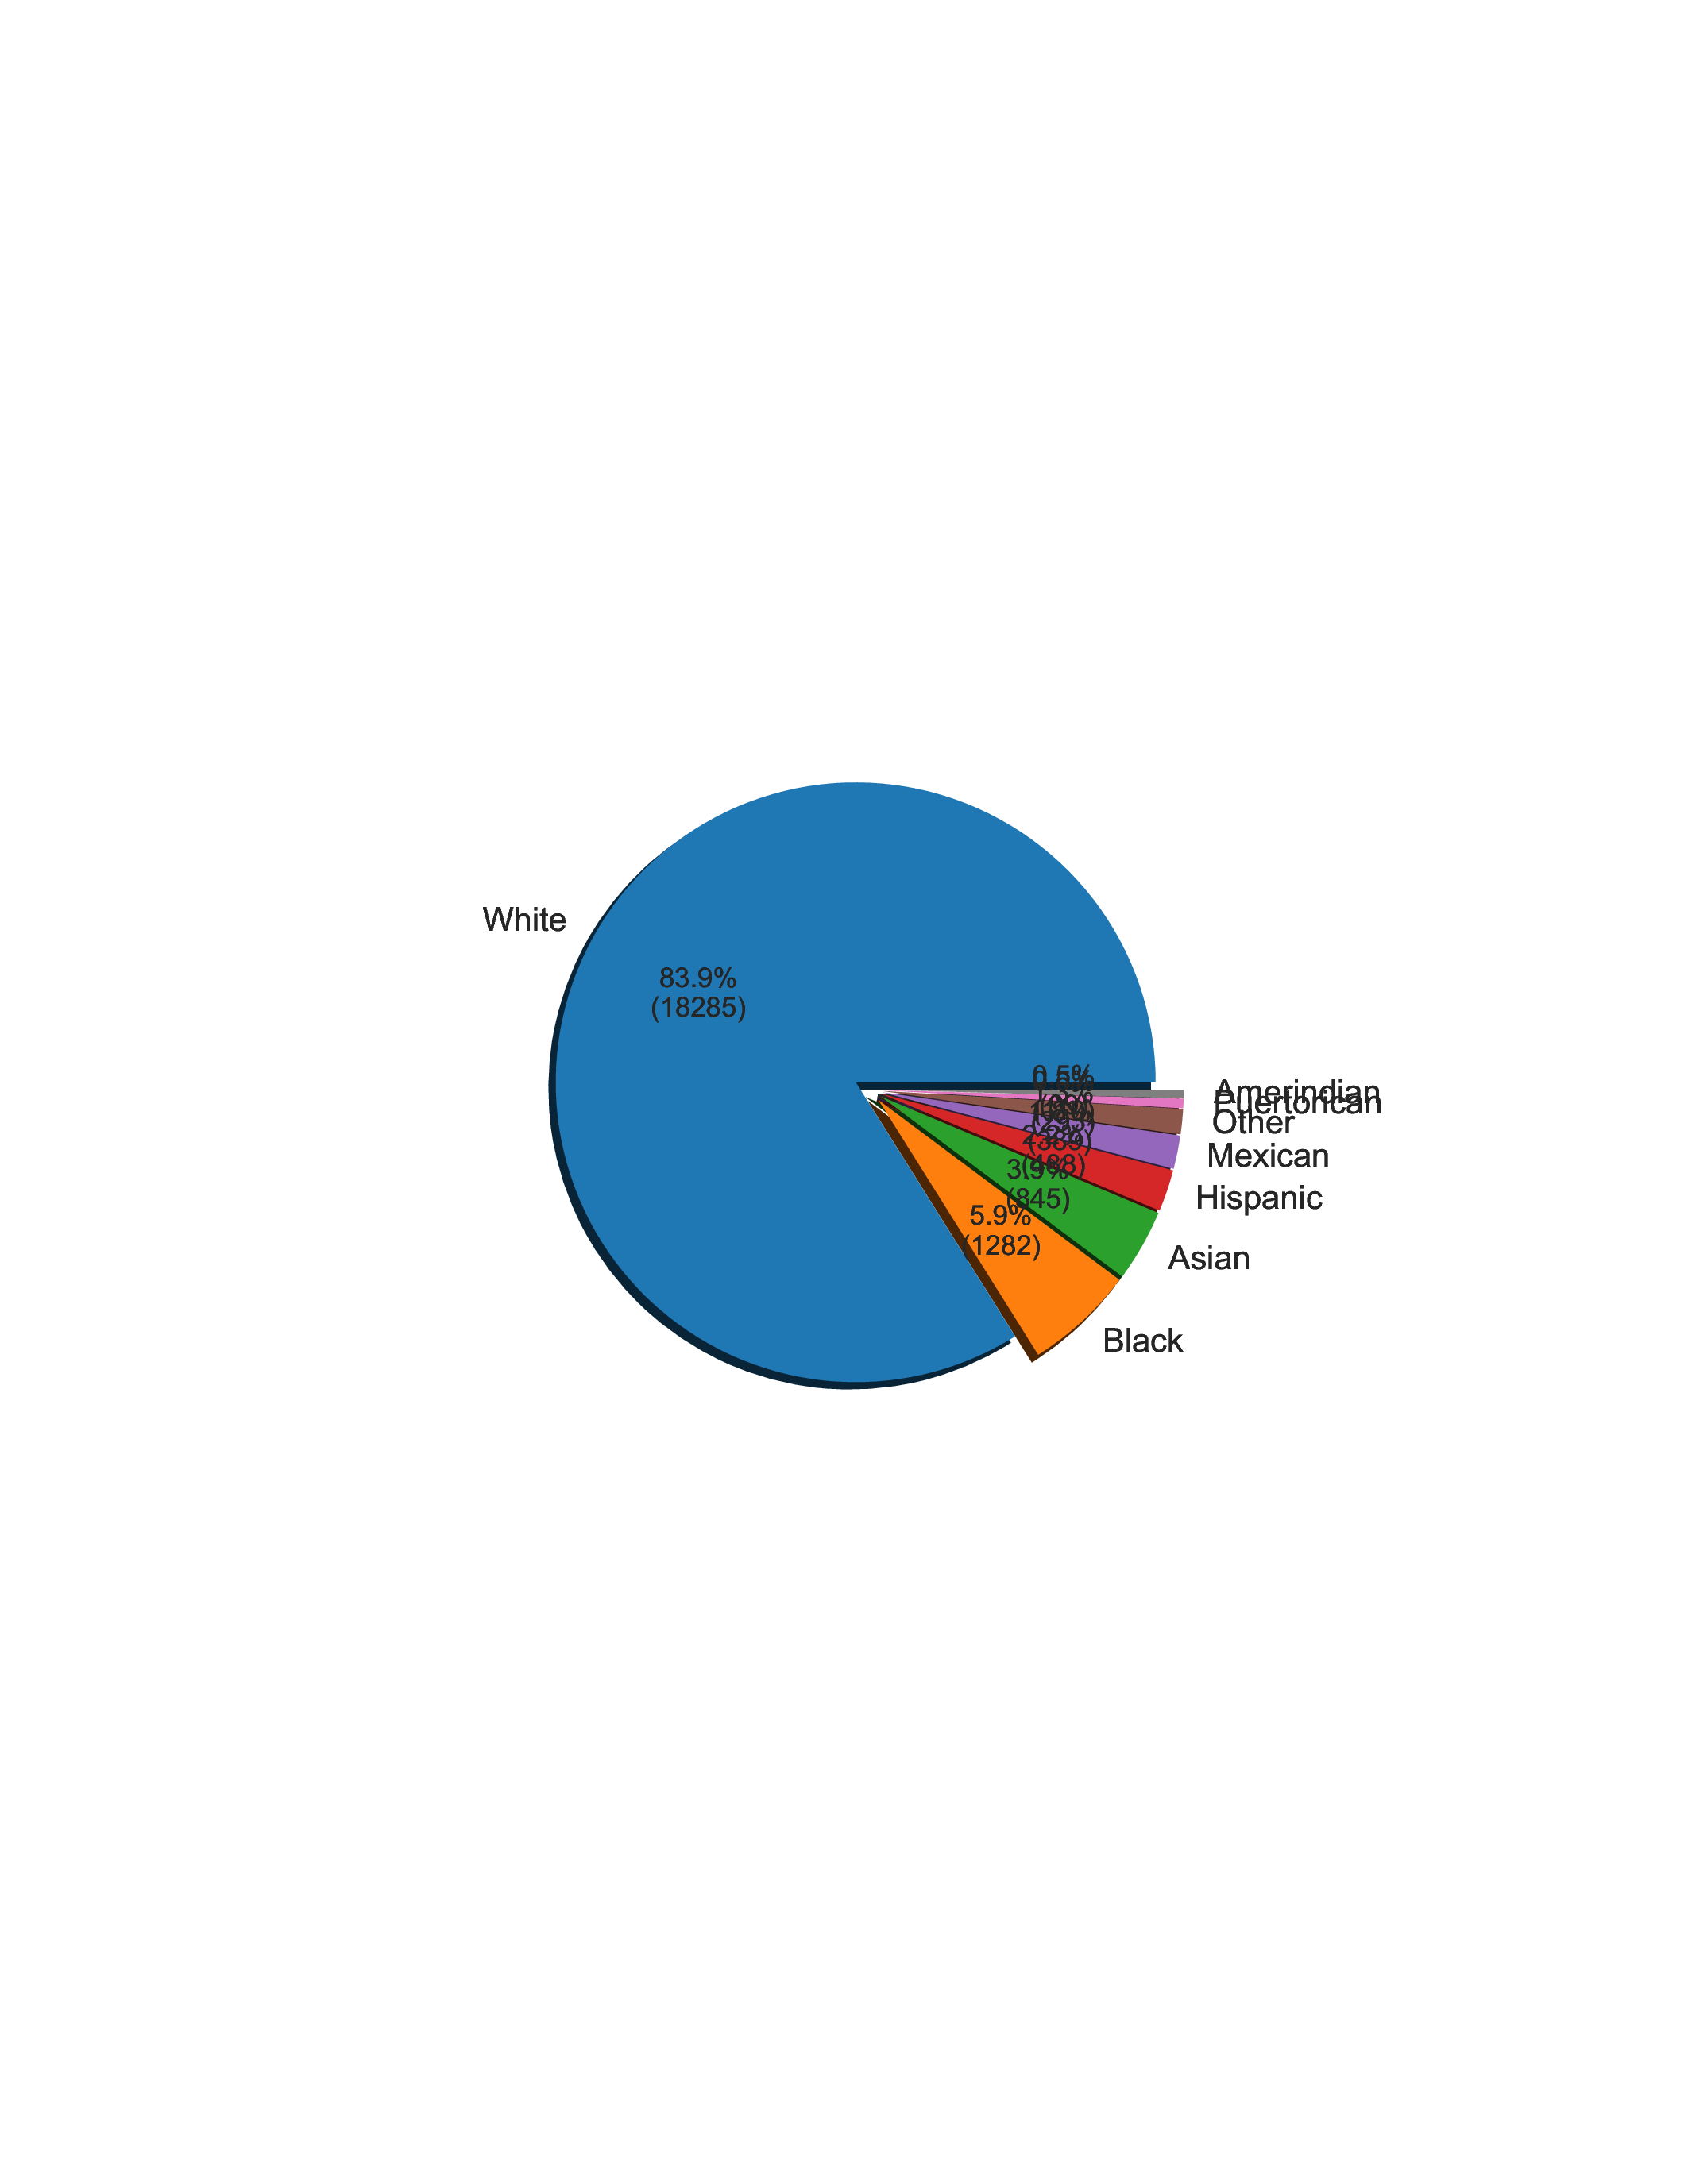}
  \caption{\textit{Race} categories distribution}
\end{subfigure}%
\begin{subfigure}{.5\textwidth}
  \centering
  \includegraphics[width=1.2\linewidth]{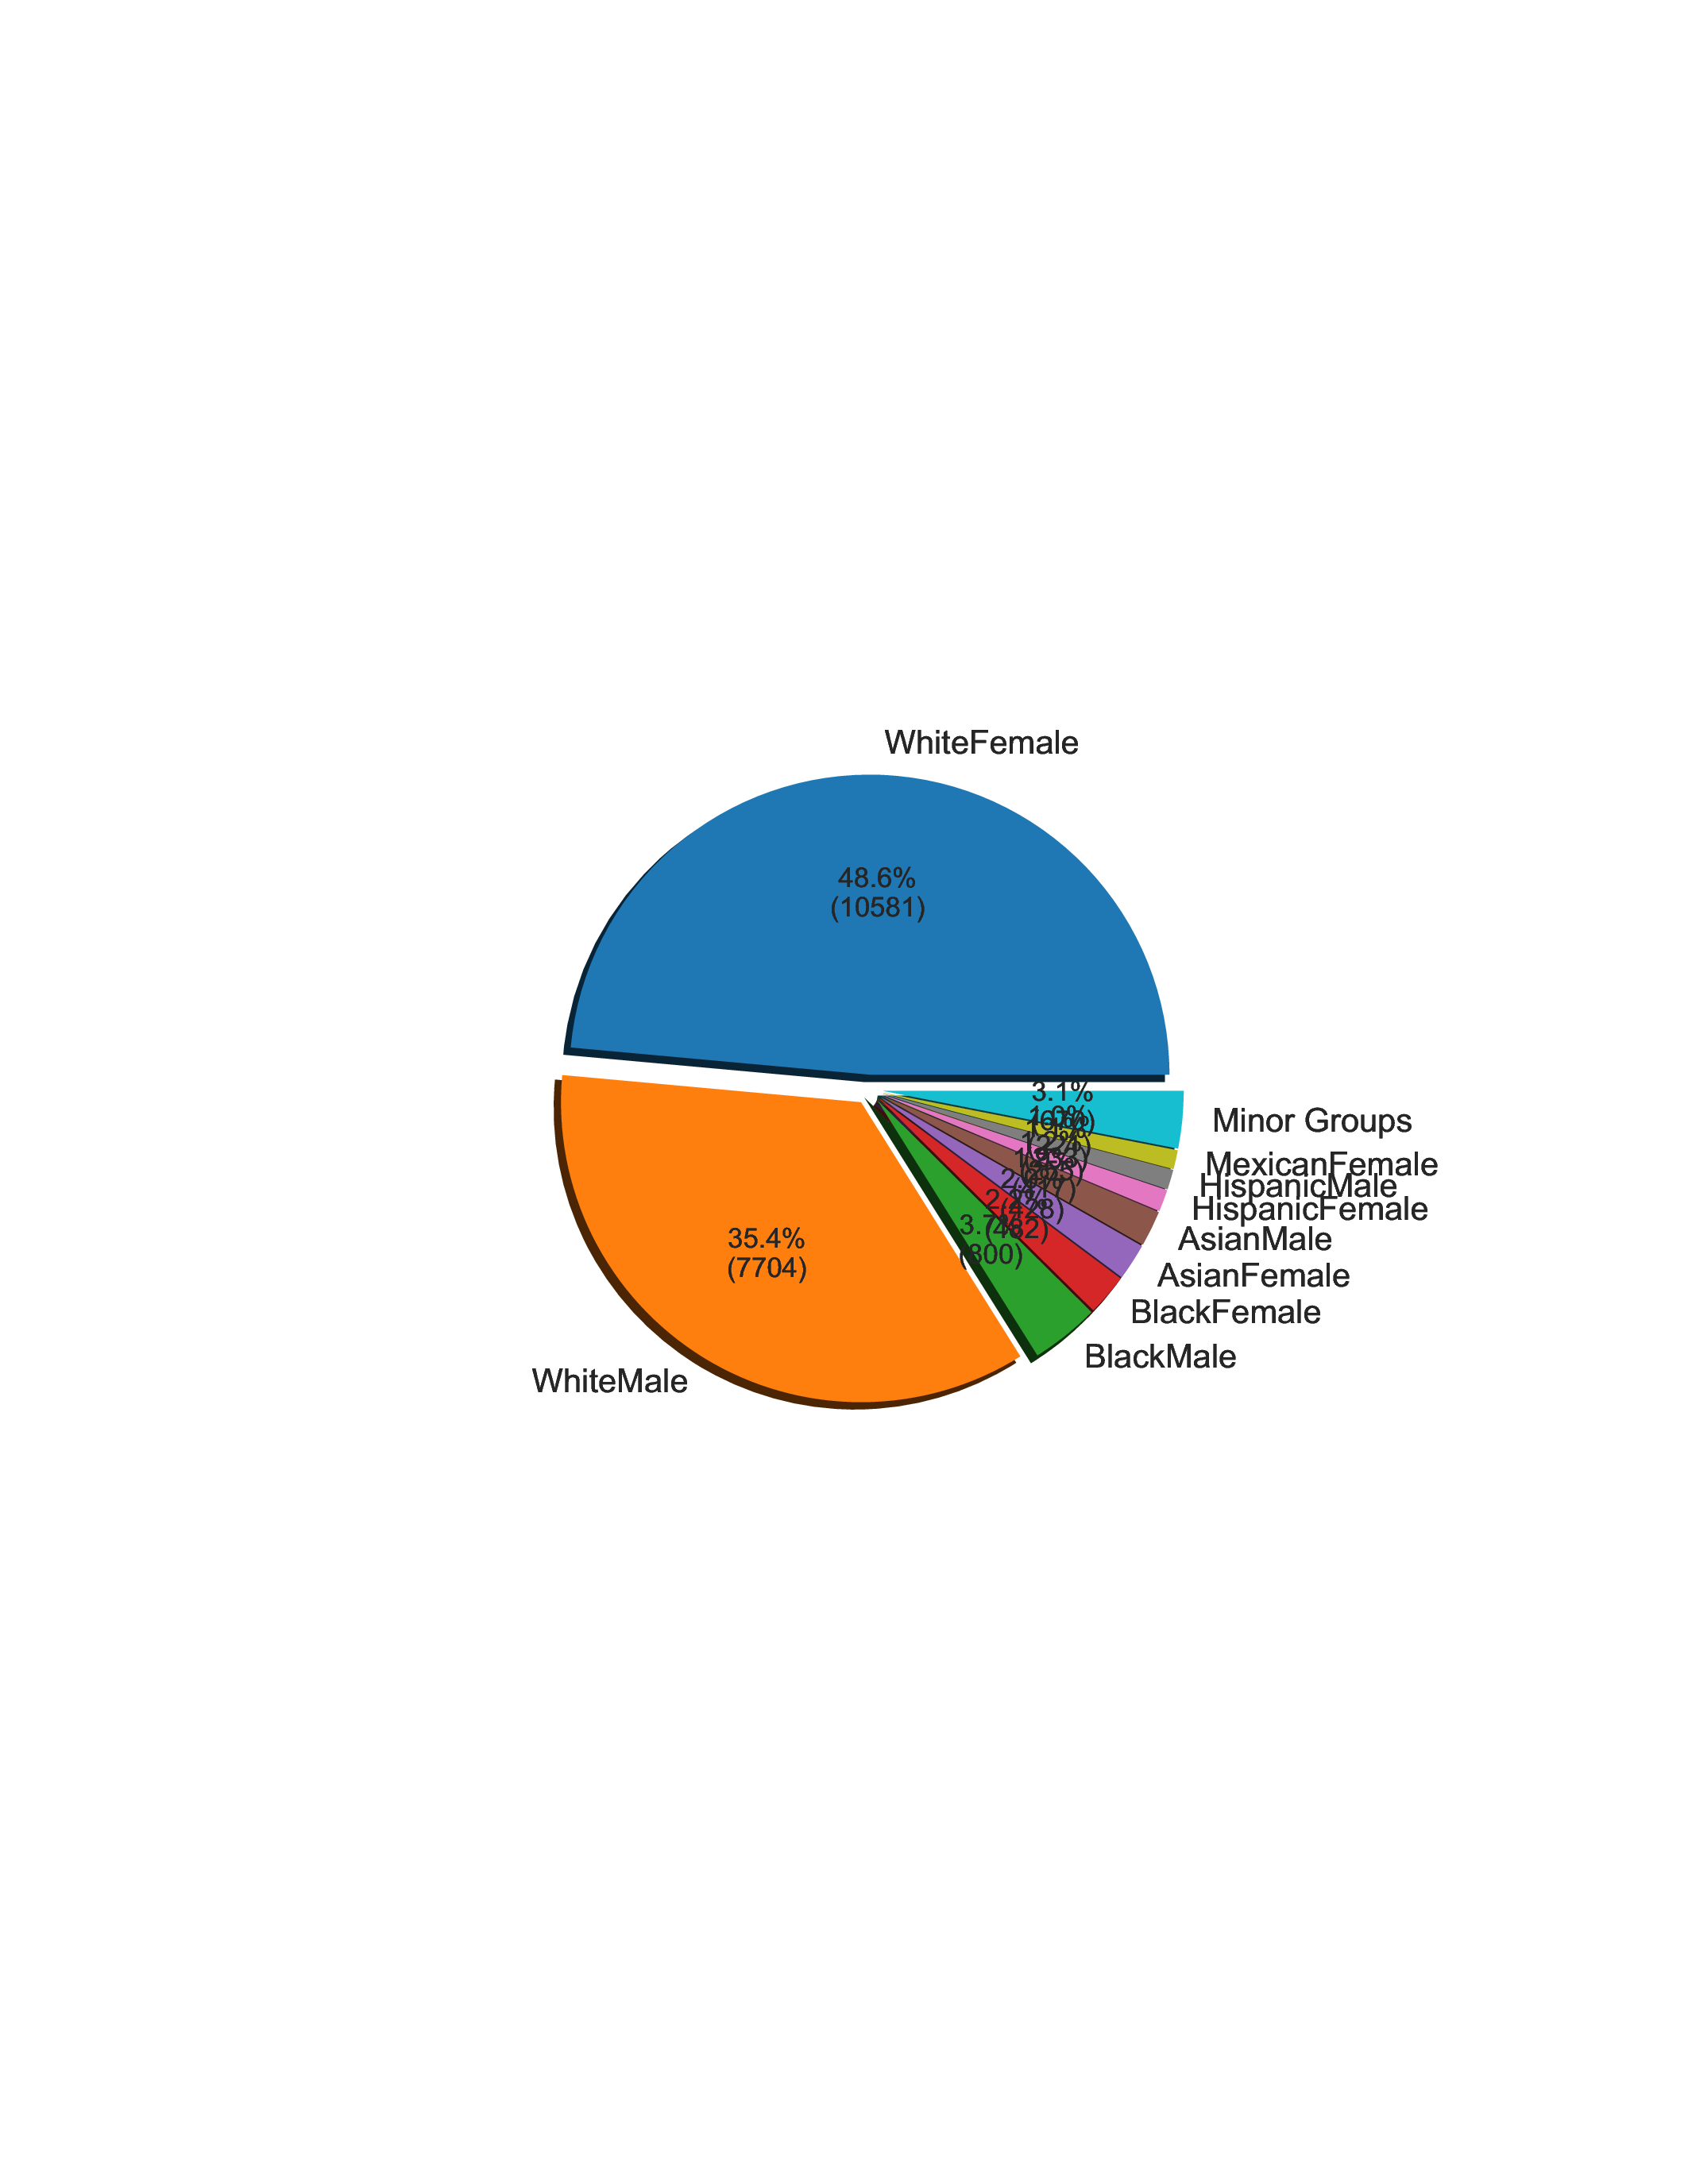}
  \caption{Intersectional fairness \textit{RaceSex} categories distribution}
\end{subfigure}
\caption{Distribution of the protected attribute categories to be encoded and regularized for the Law School Admission Council survey dataset \cite{Wightman1998_LawDataSource}}\label{fig:pieLaw}
\end{figure}

\subsubsection*{\textbf{Irreducible induced bias}}
\vspace{1cm}

%OHE = 0.65072
The irreducible bias that is induced while encoding categorical features is due to statistical differences in large groups (Section~\ref{sec:relatedwork}). For this case, we choose the two largest groups in the dataset: \textit{White} and \textit{Black}. We investigate the trade-off between equal opportunity fairness and AUC metrics while using two different encoding techniques (Section~\ref{sec:relatedwork}) and with two different regularization techniques (Section~\ref{sec:regularization}). Figure~\ref{fig:LawIrred} shows that the general loss of model performance in over parametrized cases is less than in the previous use case with COMPAS. In this case, for the smoothing regularization light hyperparameters show an increase of equal opportunity fairness, and after a plateau that can be seen in Figure \ref{fig:hyperLawSmoothing}, the regularization achieves equal opportunity fairness. 

From Figures~\ref{fig:hyperLawGaus} and \ref{fig:hyperLawSmoothing}, we can see how the drop in model performance is almost negligible, but the equal opportunity fairness is disparate, ranging in its absolute maximum values $[0,1]$. In Figure \ref{fig:LawIrred}, we observe that the smoothing regularization during the first values increases the discrimination and after a plateau in fairness eventually improves and decreases discrimination. Under a stronger regularization, we reach an equal opportunity treatment between White and African-American groups. Further details about the changes in model performance and fairness can be seen in Figures \ref{fig:hyperLawSmoothing} and \ref{fig:hyperLawGaus}, where we observe similar trends. %\sr{Bad English. Restructure paragraph. State what the figures report, and how to read them to conclude.}

\begin{figure}[ht]
    \centering
    \includegraphics[width=0.8\linewidth]{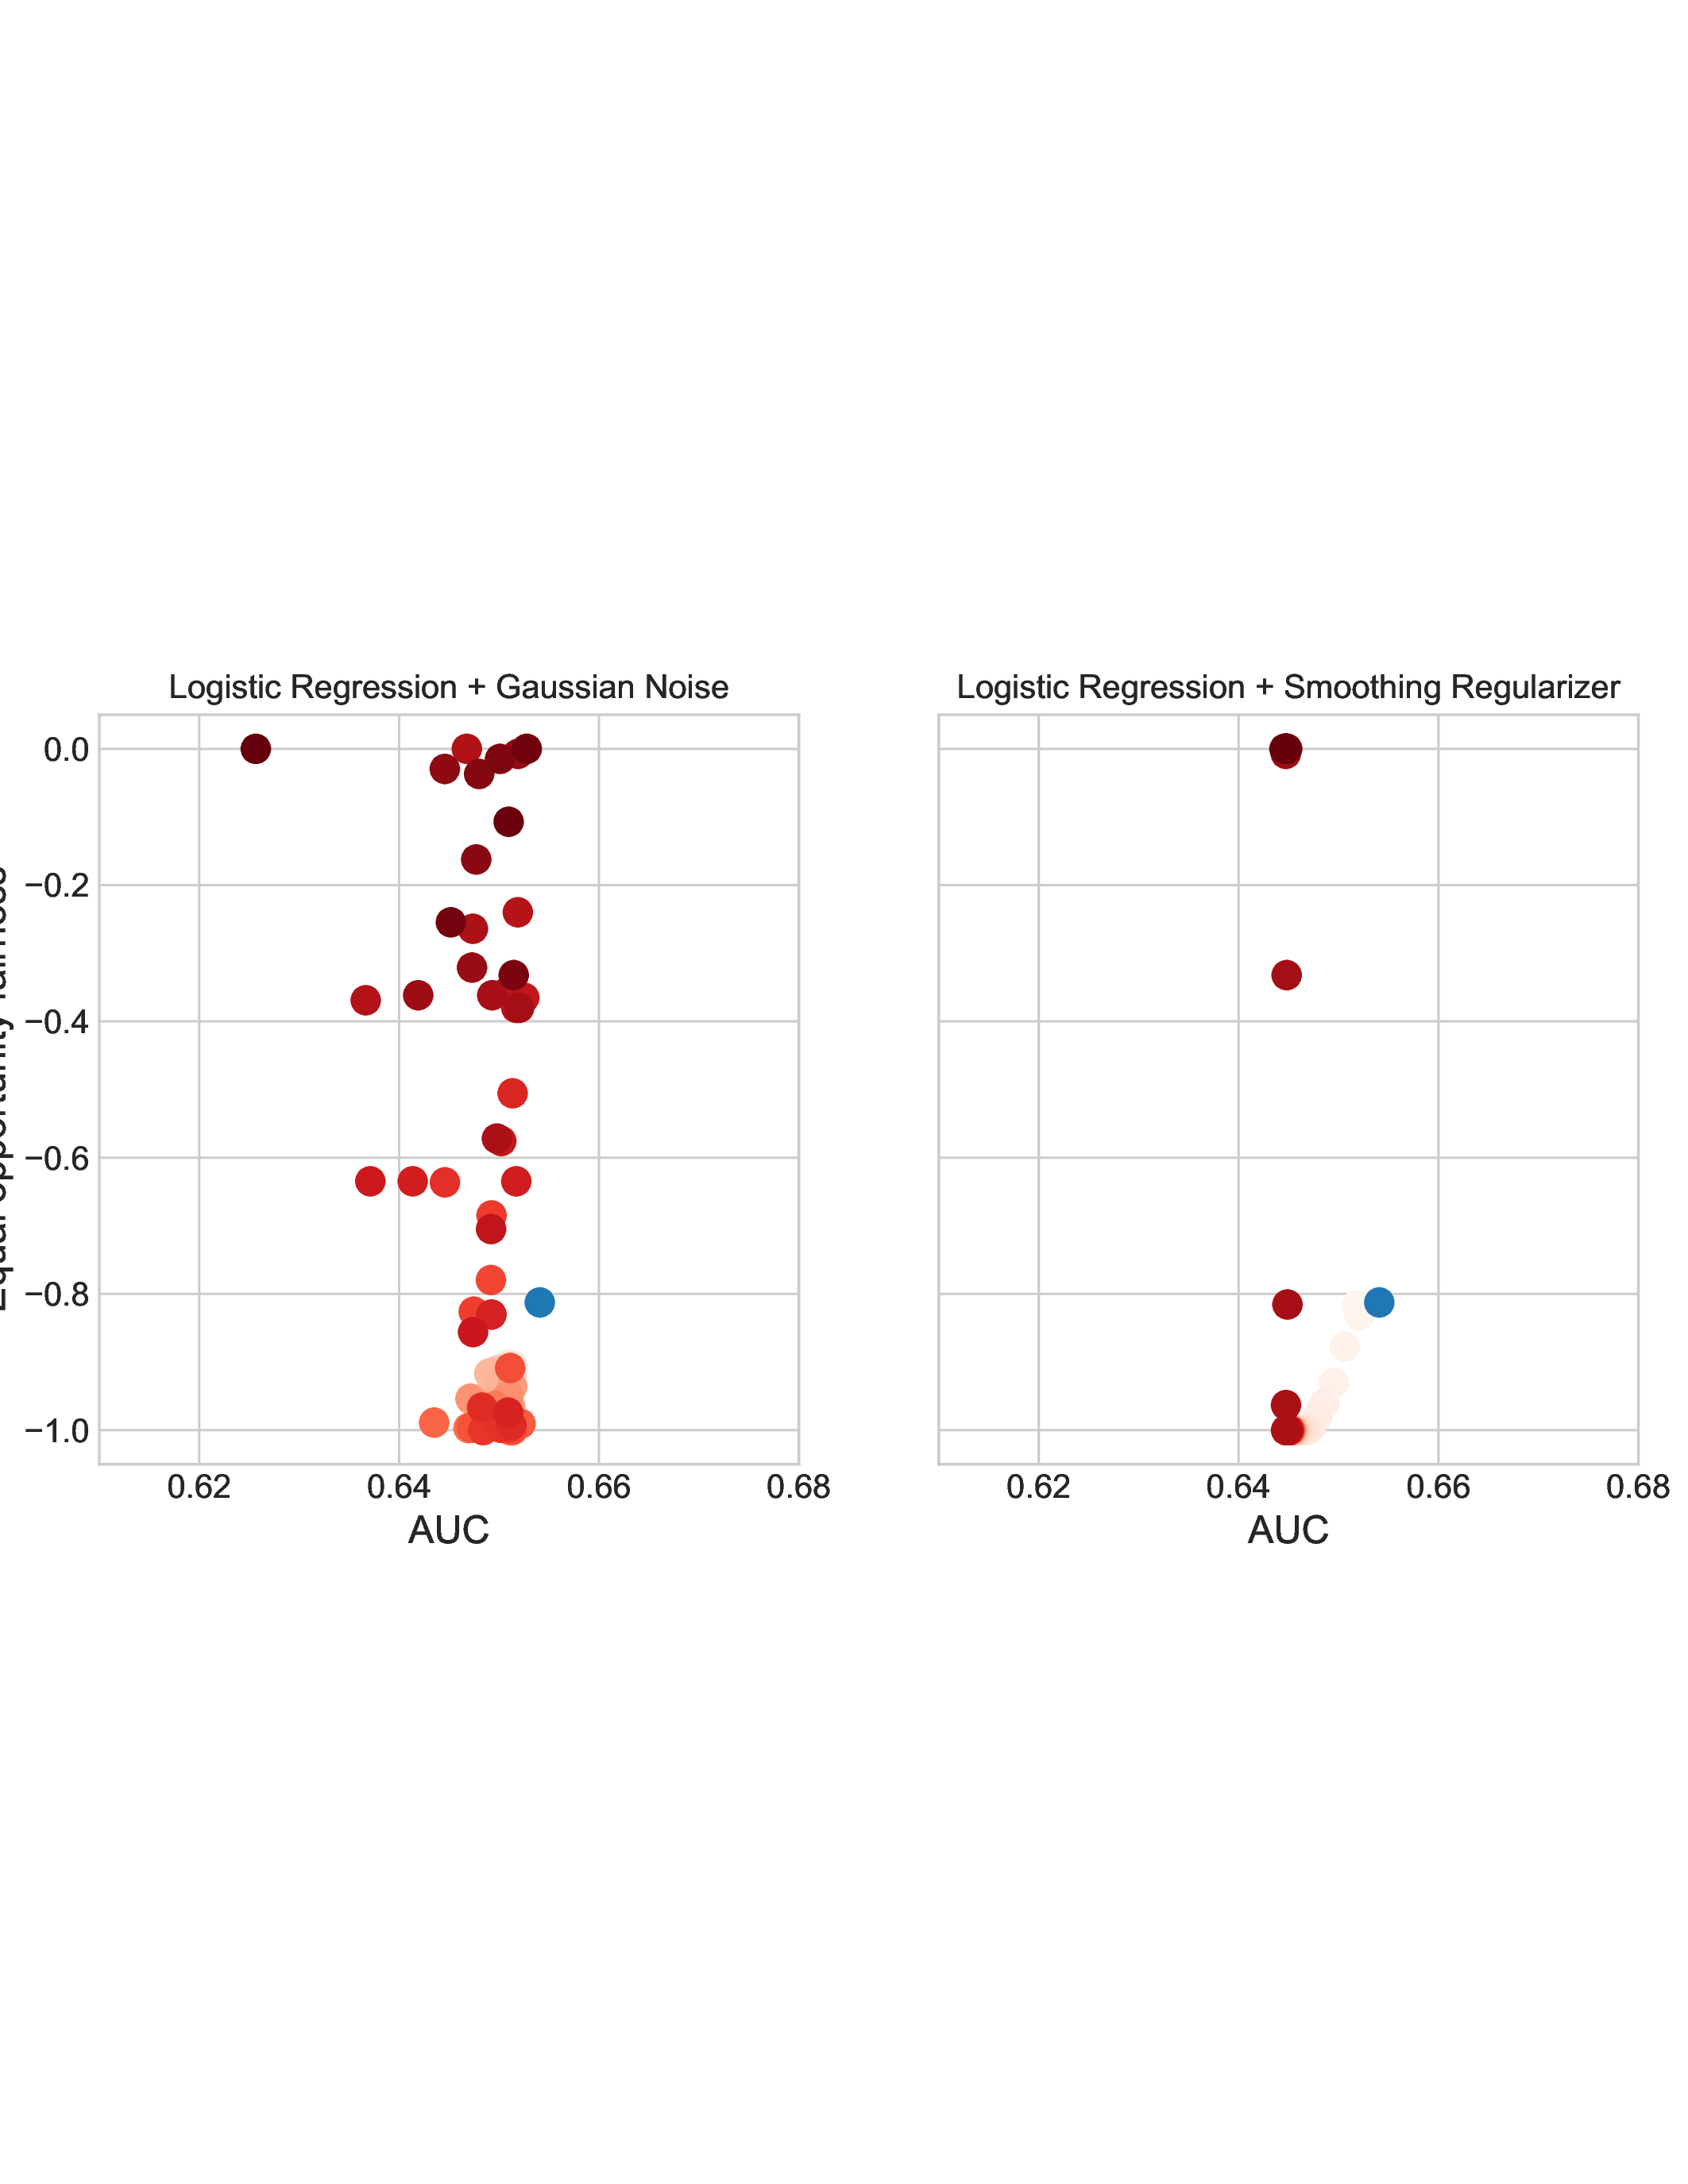}
    \caption{Comparing one-hot encoding and target encoding regularization (Gaussian noise and smoothing) for the Logistic Regression over the test set of the Law School Admission Council survey dataset. Protected group is \textit{Black}. Reference group is \textit{White}. Red dots regard different regularization parameters: the darker the red the higher the regularization. Blue dot regards the one-hot encoding.}
    \label{fig:LawIrred}
\end{figure}

\begin{figure}[ht]
    \centering
    \includegraphics[width=0.8\linewidth]{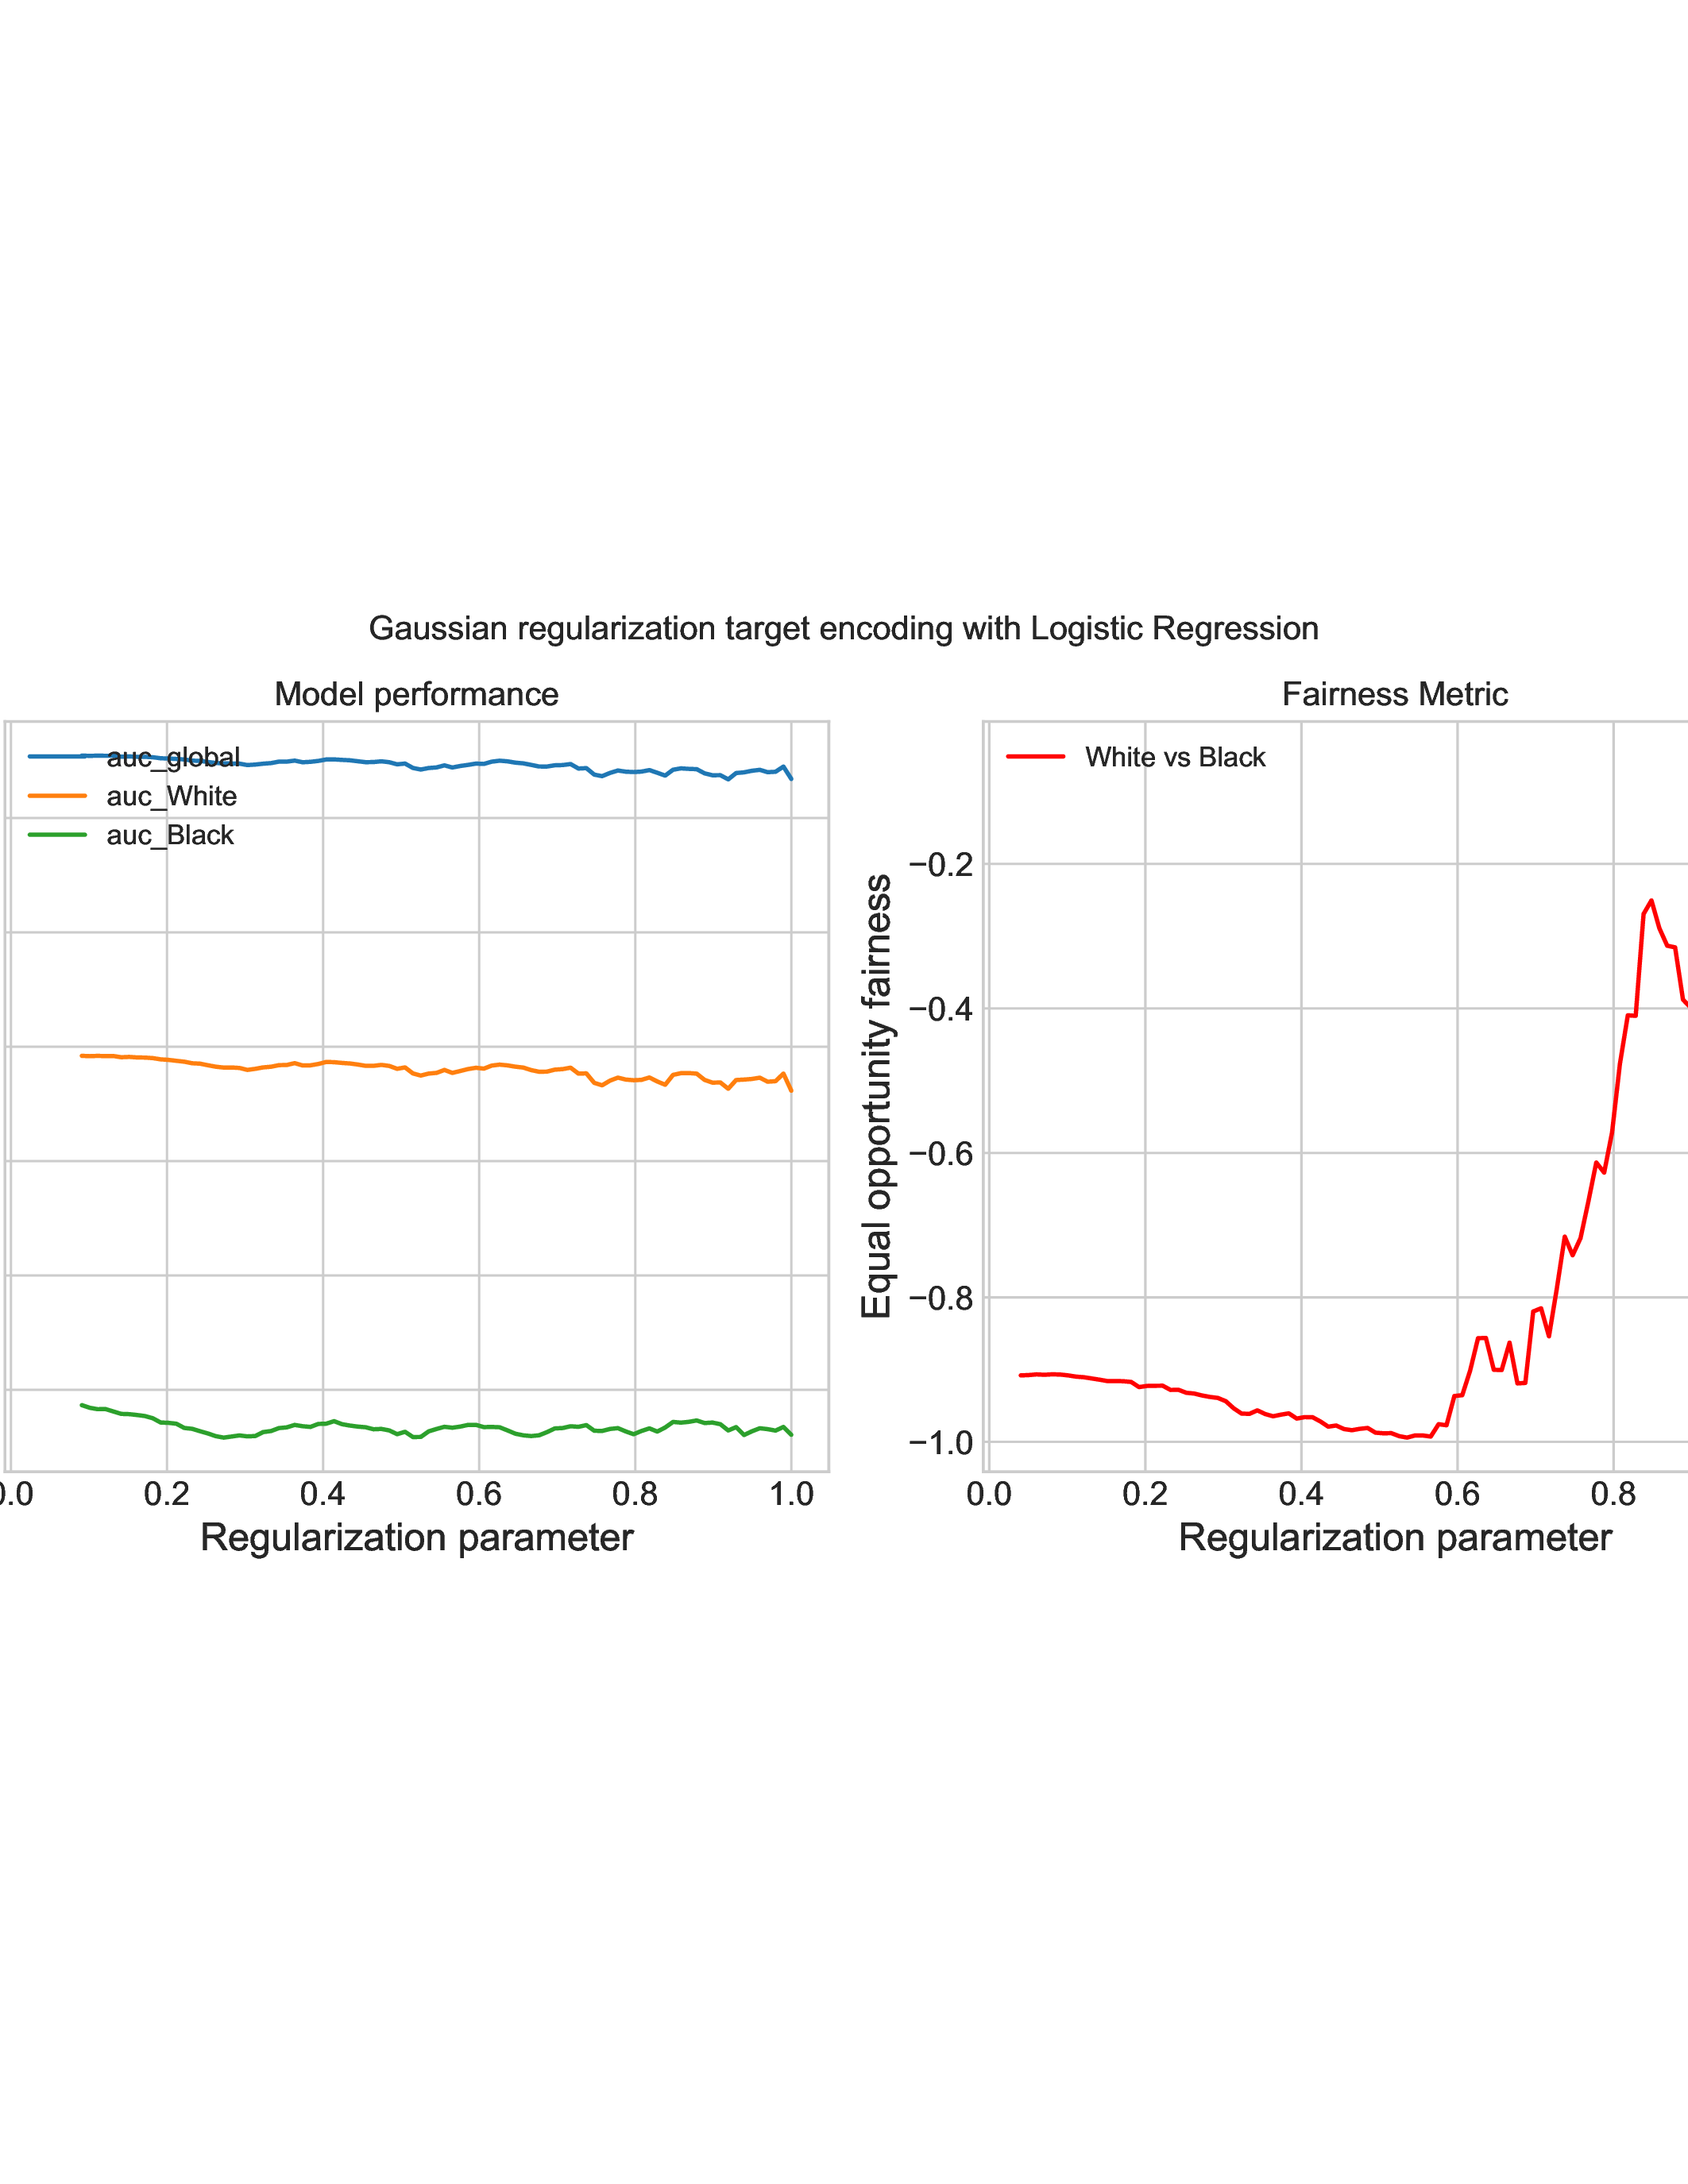}
    \caption{Impact of the Gaussian noise regularization parameter $\lambda$ on performance and fairness metrics over the test set of the Law School Admission Council survey dataset. In the left image the AUC of the protected group, reference group, and global over the regularization hyperparameter. On the right, the equal opportunity fairness variation throughout the regularization hyperparameter.}
    \label{fig:hyperLawGaus}
\end{figure}

\begin{figure}[ht]
    \centering
    \includegraphics[width=0.8\linewidth]{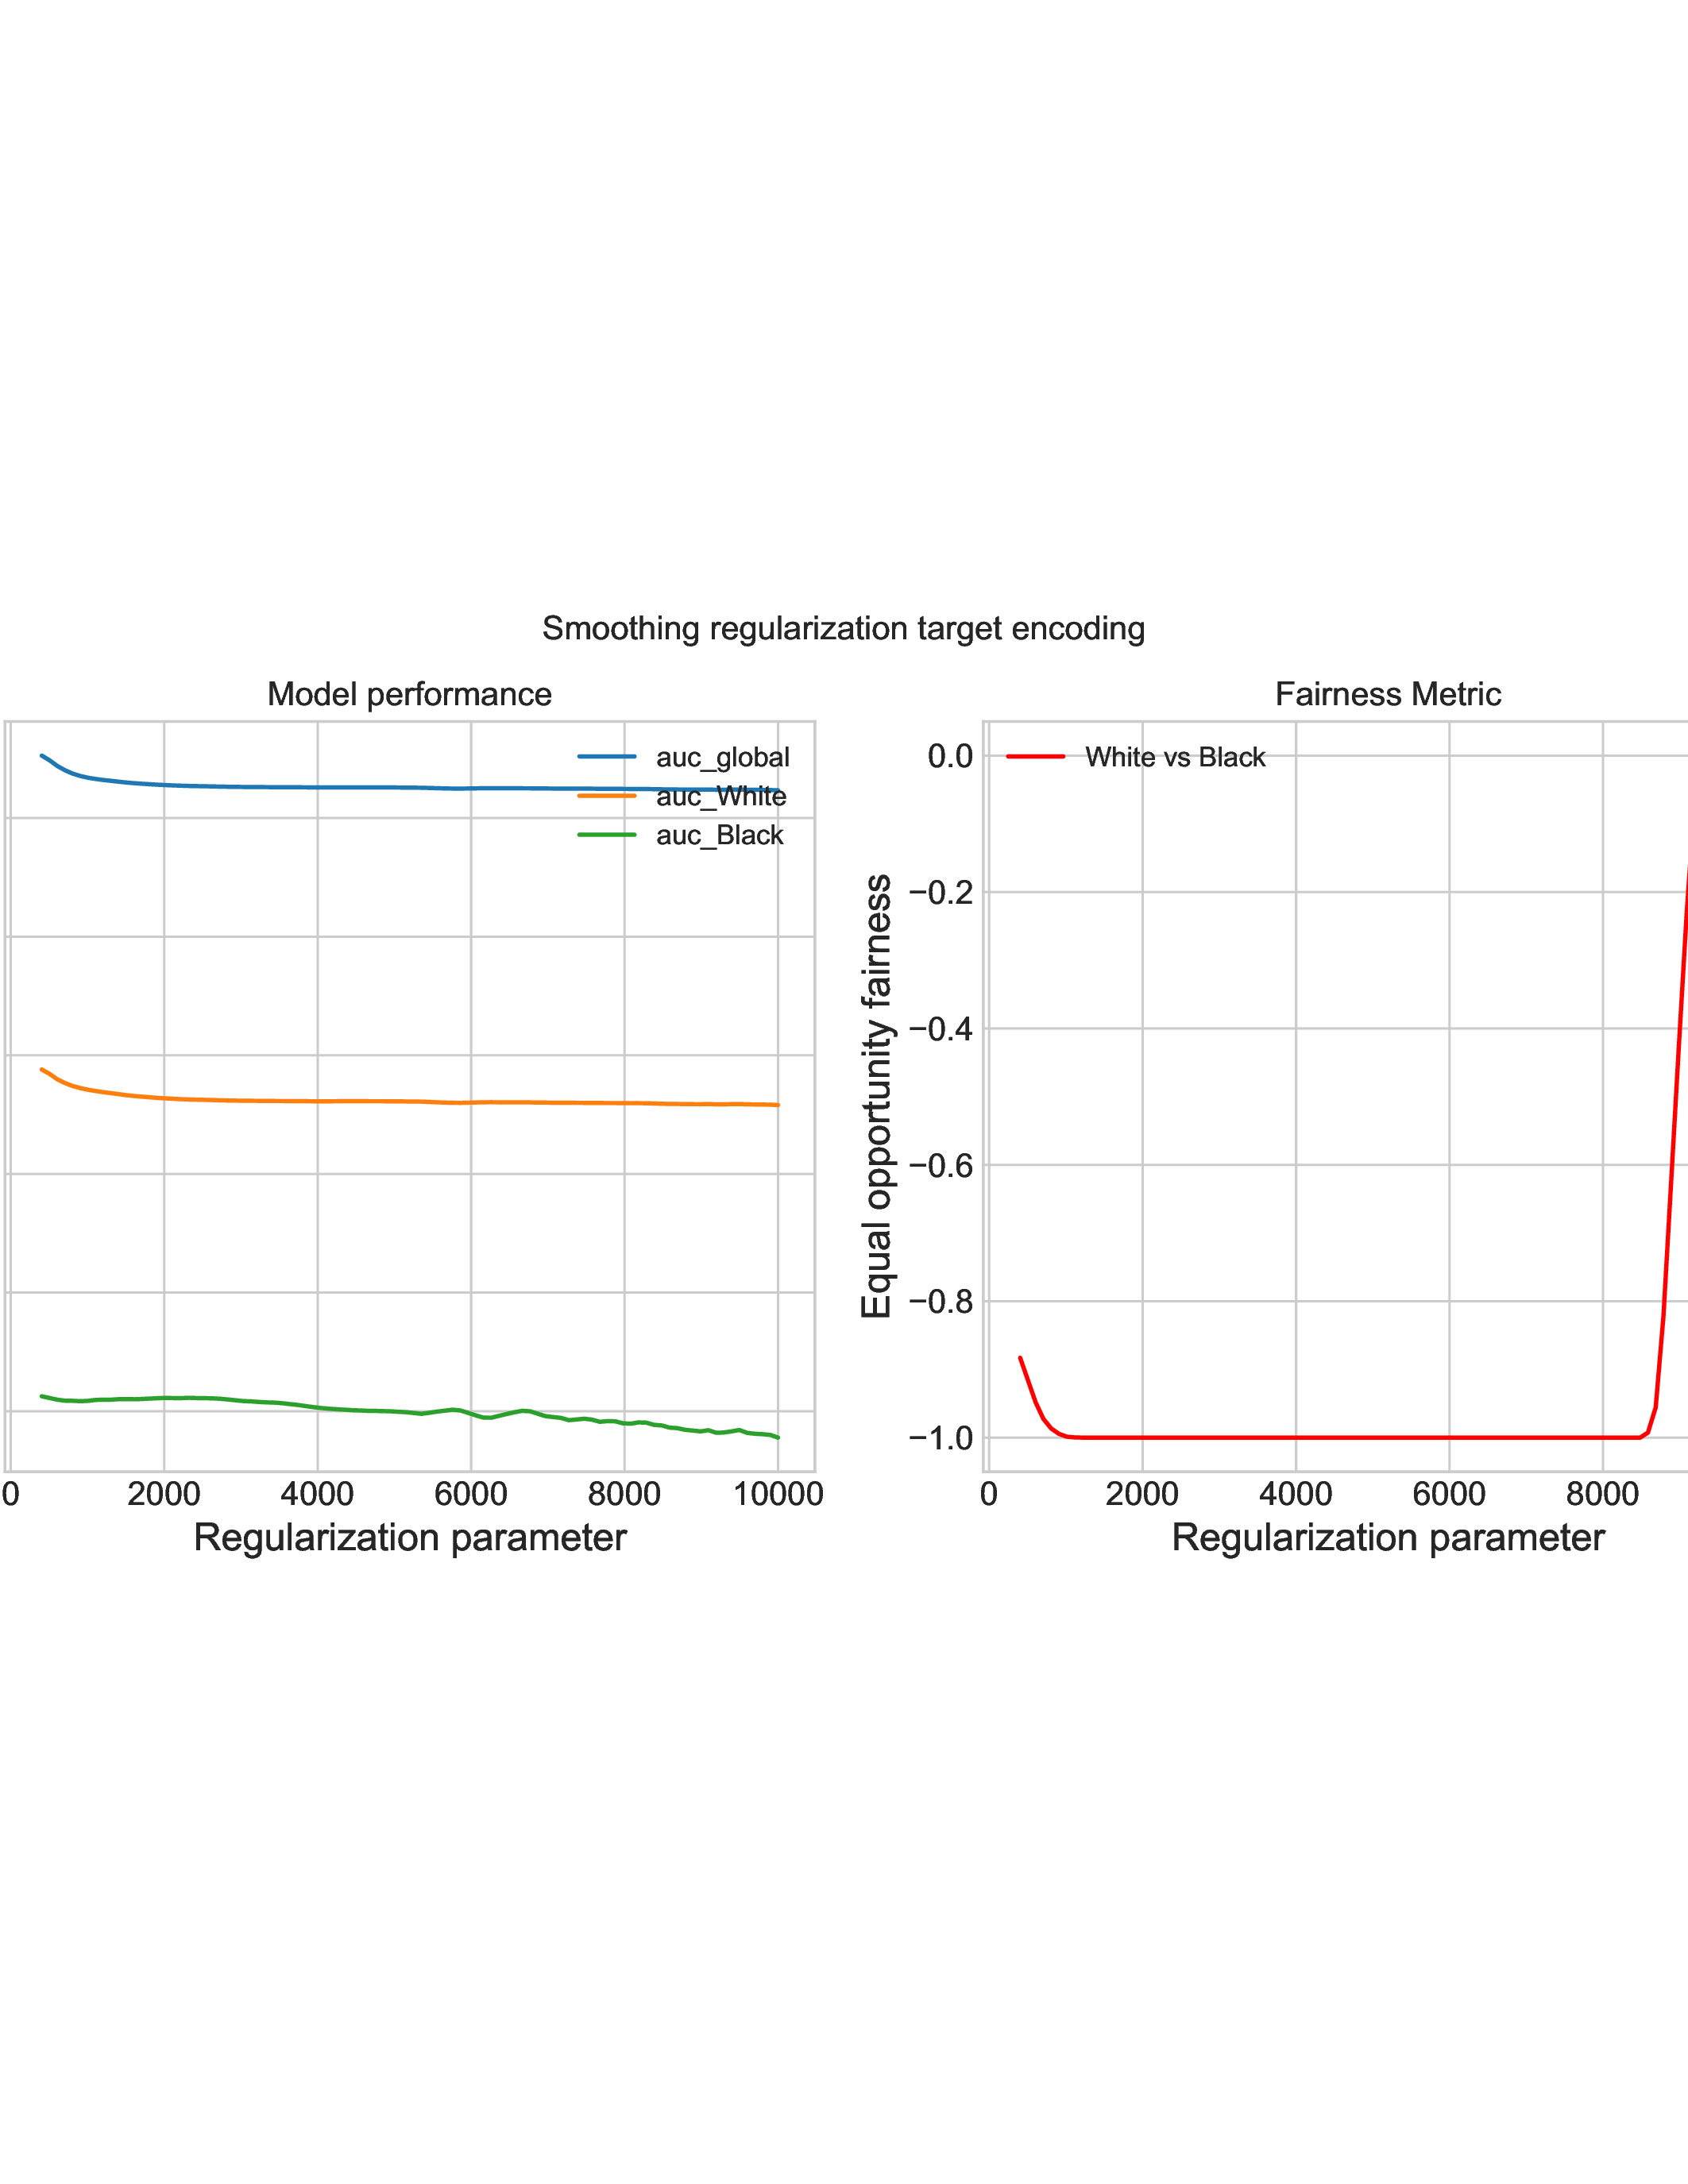}
    \caption{Impact of the smoothing regularization parameter $m$ in $\lambda(n_i) = n_i/(n_i+m)$ on performance and fairness metrics over the test set of the Law School Admission Council survey dataset. In the left image the AUC of the protected group, reference group and global over the regularization hyperparameter. On the right, the equal opportunity fairness variation through out the regularization hyperparameter.}
    \label{fig:hyperLawSmoothing}
\end{figure}

\subsubsection*{\textbf{Reducible induced bias}}
\vspace{1cm}

For induced reducible bias, that arises due to the large variance found when sampling small groups. To replicate this biased situation, from the most common ethnic group, \textit{White}, we sample a $\approx 0.005$ fraction, being the ratio of $120$ against $22,000$  samples (cf. Figure \ref{fig:pieLaw}). We treat this sampled group as the protected group and the original \textit{White}. Both come from the same distribution so if we had enough statistical mass for both of them, the encoding should be the same. It is worth noting that due to the stochastic nature of this sampling experiment, different randomization seeds will produce different results. For this particular split, the mean of the sampled group is $0.16$ while the reference group has a mean of $0.59$. The regularization hyperparameters are the same as in the previous experiment (Section~\ref{exp:first}).

\begin{figure}[ht]
    \centering
    \includegraphics[width=0.8\linewidth]{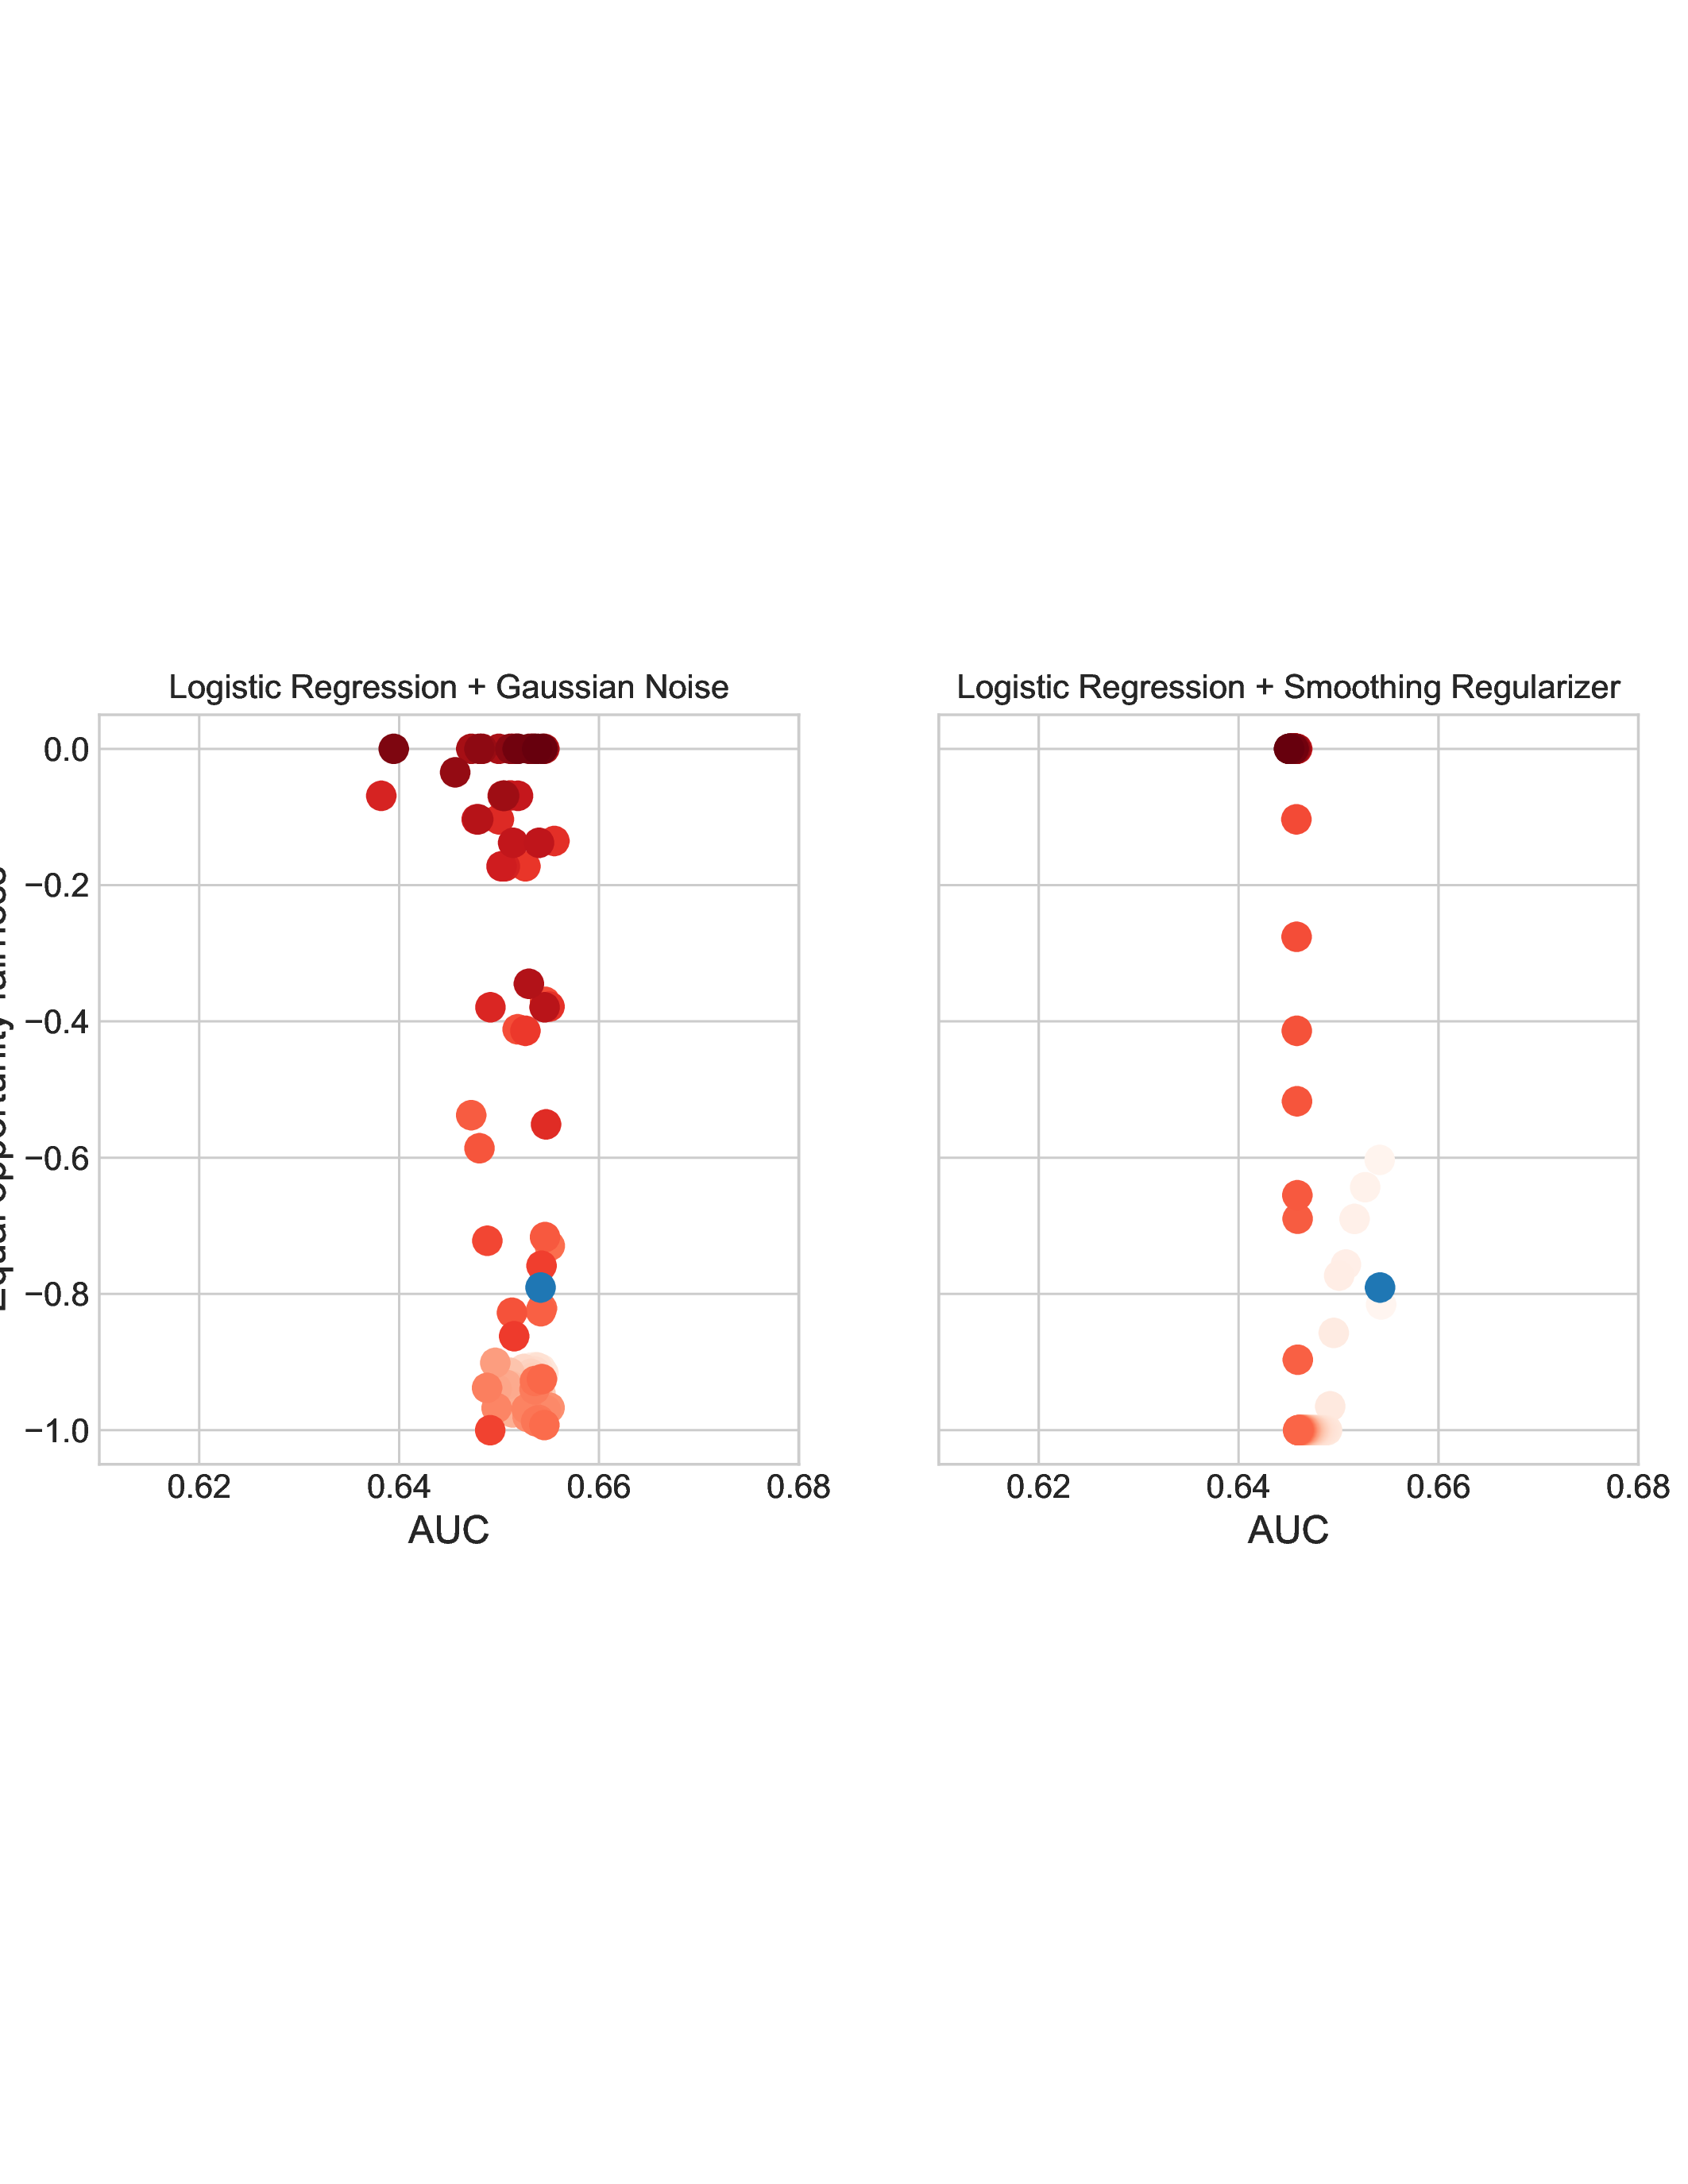}
    \caption{Comparing one-hot encoding and target encoding regularization (Gaussian noise and smoothing) for the Logistic Regression over the test set of the Law School Admission Council survey dataset. Reference group is \textit{White}. Protected group is a $0.005$ sample of \textit{White}. Red dots regard different regularization parameters: the darker the red the higher the regularization. Blue dot regards the one-hot encoding.}
    \label{fig:LawRed}
\end{figure}

\begin{figure}[ht]
    \centering
    \includegraphics[width=0.8\linewidth]{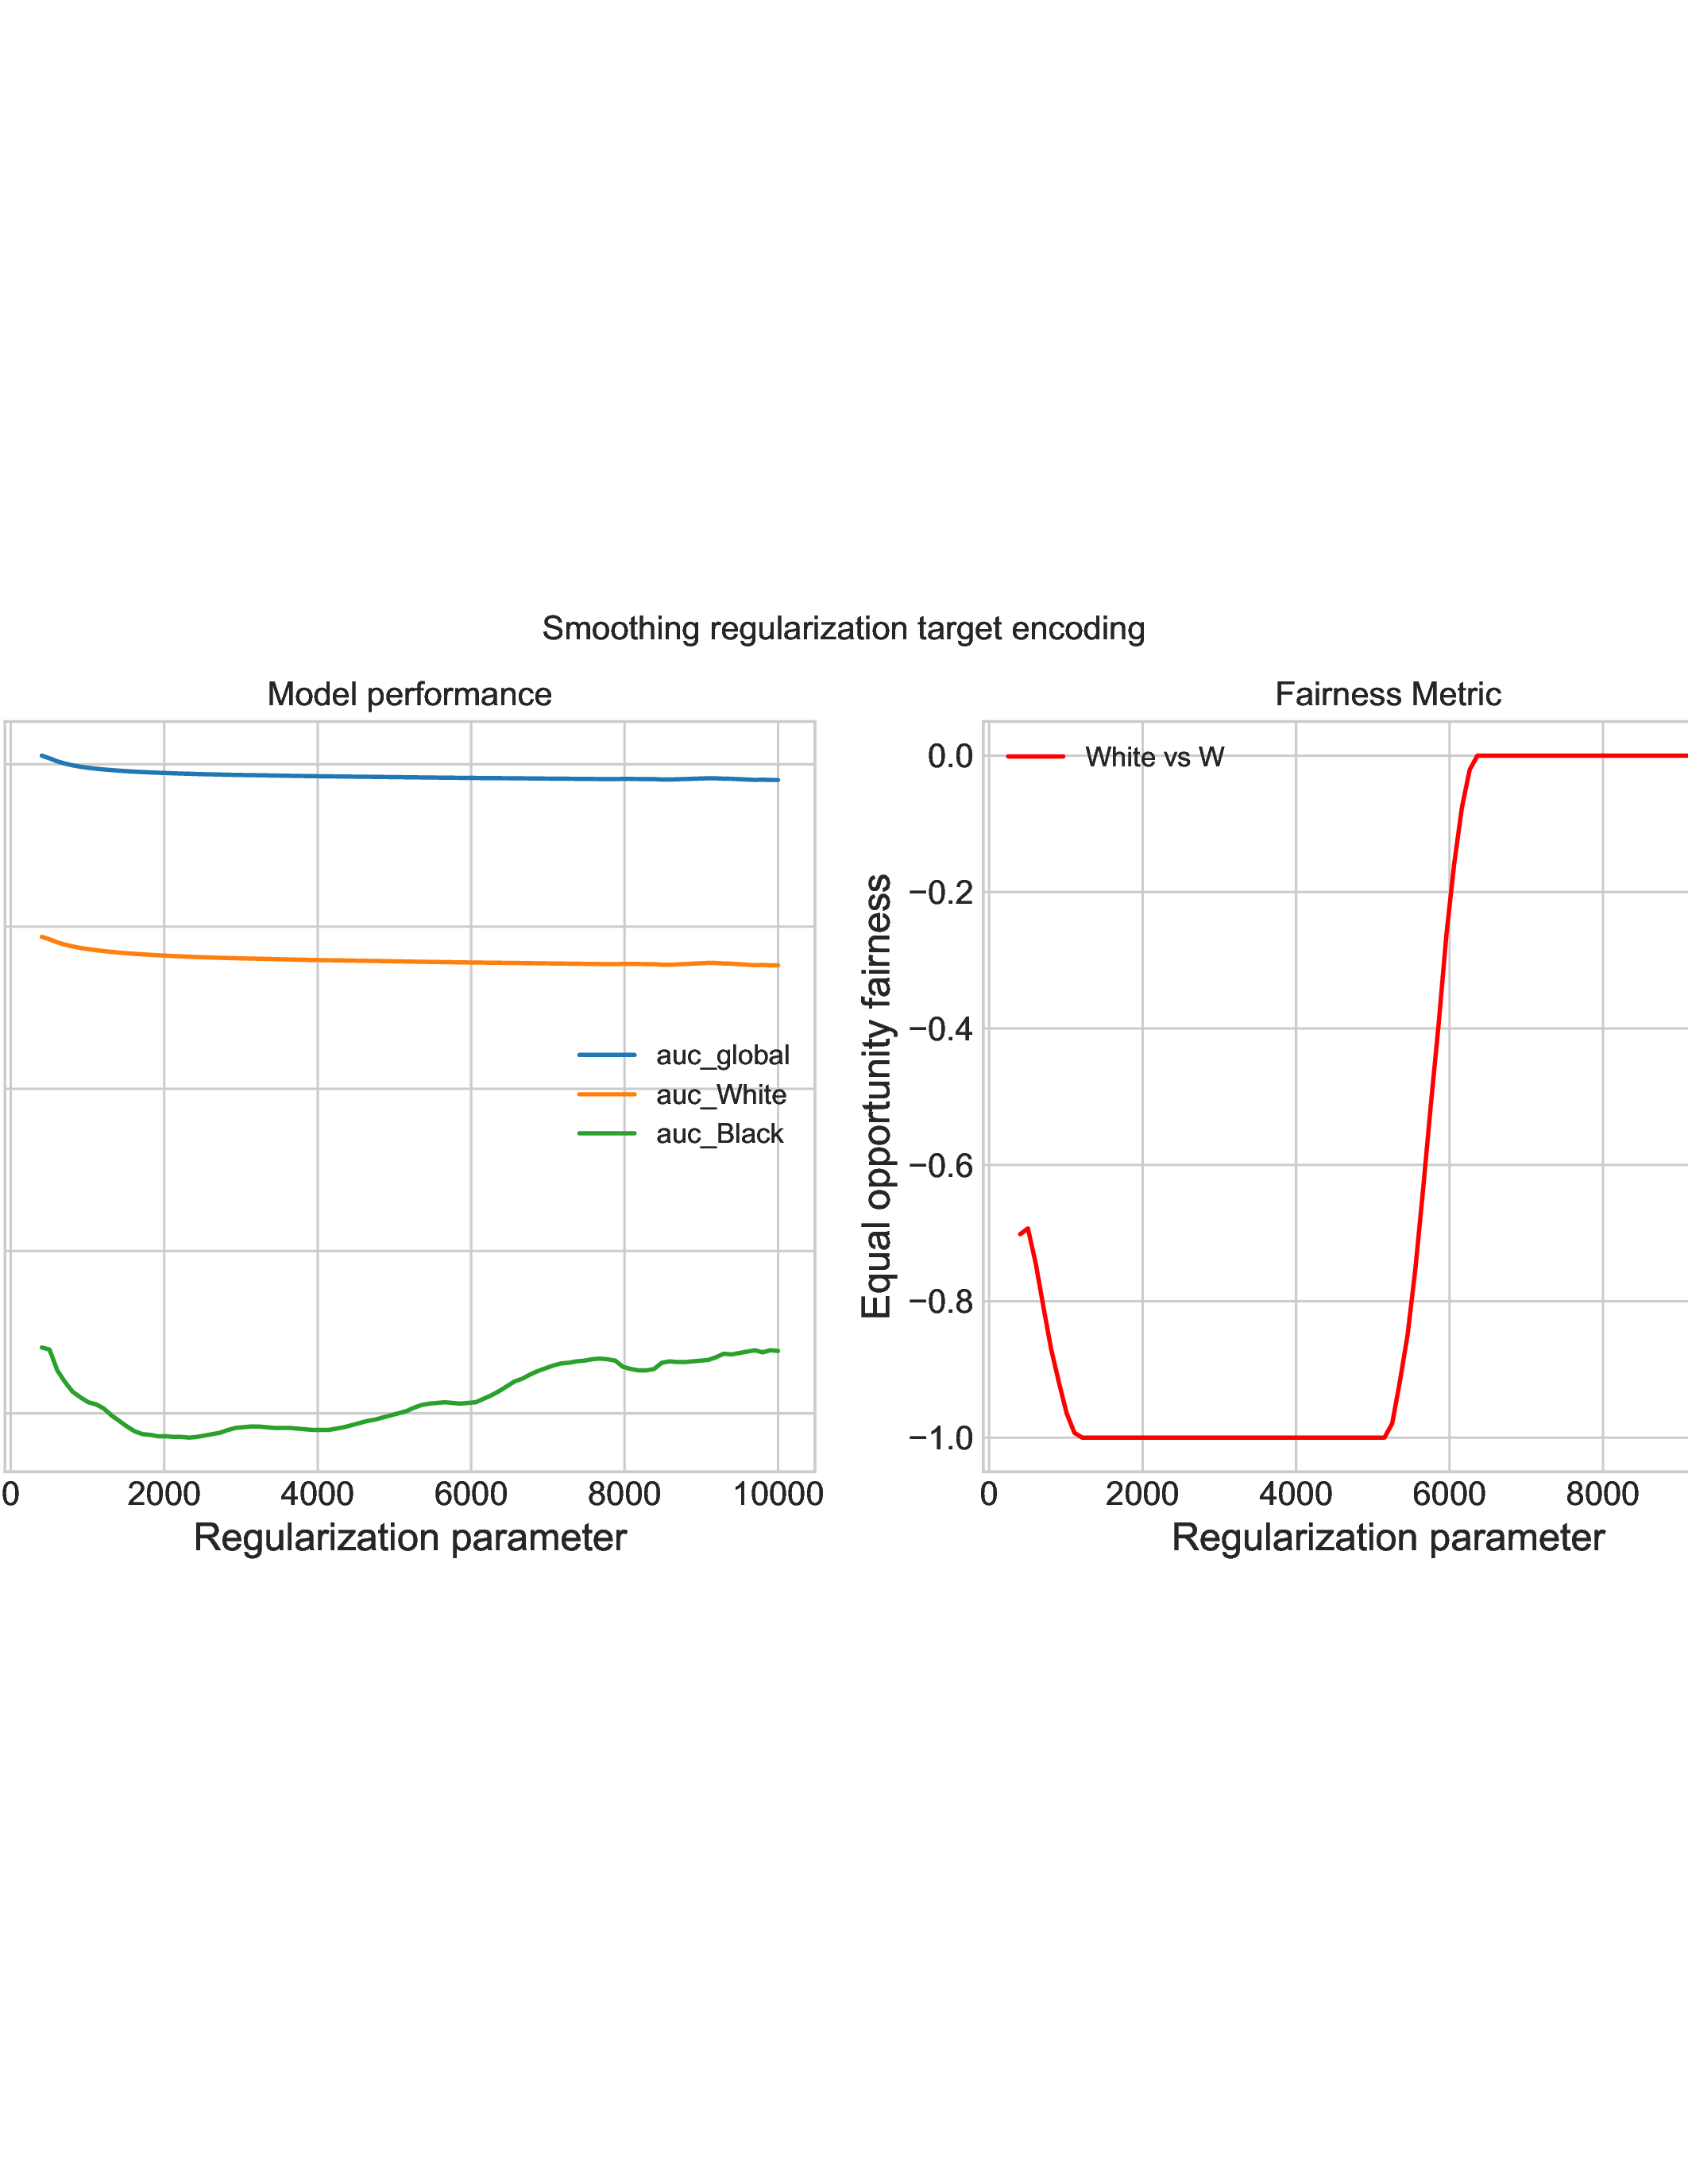}
    \caption{Impact of the smoothing regularization parameter $m$ in $\lambda(n_i) = n_i/(n_i+m)$ under reducible fairness comparison, on performance and fairness metrics over the test set of the Law School Admission Council survey dataset. In the left image the AUC of the protected group, reference group and global over the regularization hyperparameter. On the right, the equal opportunity fairness variation through out the regularization hyperparameter.}
    \label{fig:hyperLawSmoothingRed}
\end{figure}
In Figure \ref{fig:LawRed}, we can see a logistic regression estimator that is fed encoded variables in the two different encoding ways. Non-regularized target encoding is more discriminant than one-hot encoding and the AUC is almost the same with negligible differences. For both regularizations, the model performance does not vary, but the fairness does so significantly. The main difference of the experiments on Law and COMPAS datasets is that model performance variations, the fairness is correctly regularized in both cases.  One noticeable difference between reducible and irreducible induced bias experiment under smoothing regularization is that it needs less tuning of hyperparameter, lighter red dots in Figures (\ref{fig:LawIrred}) and (\ref{fig:LawRed}) or directly comparing the size of the hyperparameter plateau in Figure~\ref{fig:hyperLawSmoothing} vs Figure~\ref{fig:hyperLawSmoothingRed}.

\subsubsection*{\textbf{Intersectionality on Law}}

For this intersectional fairness experiment we concatenate \textit{Race} and \textit{Sex} status of the Law School Admission dataset.  We select \textit{Black Female} as the protected group and \textit{White Male} as the reference group. Both groups have enough statistical mass so the induced bias is not due to variance but rather it is irreducible bias.

\begin{figure}[ht]
    \centering
    \includegraphics[width=0.8\linewidth]{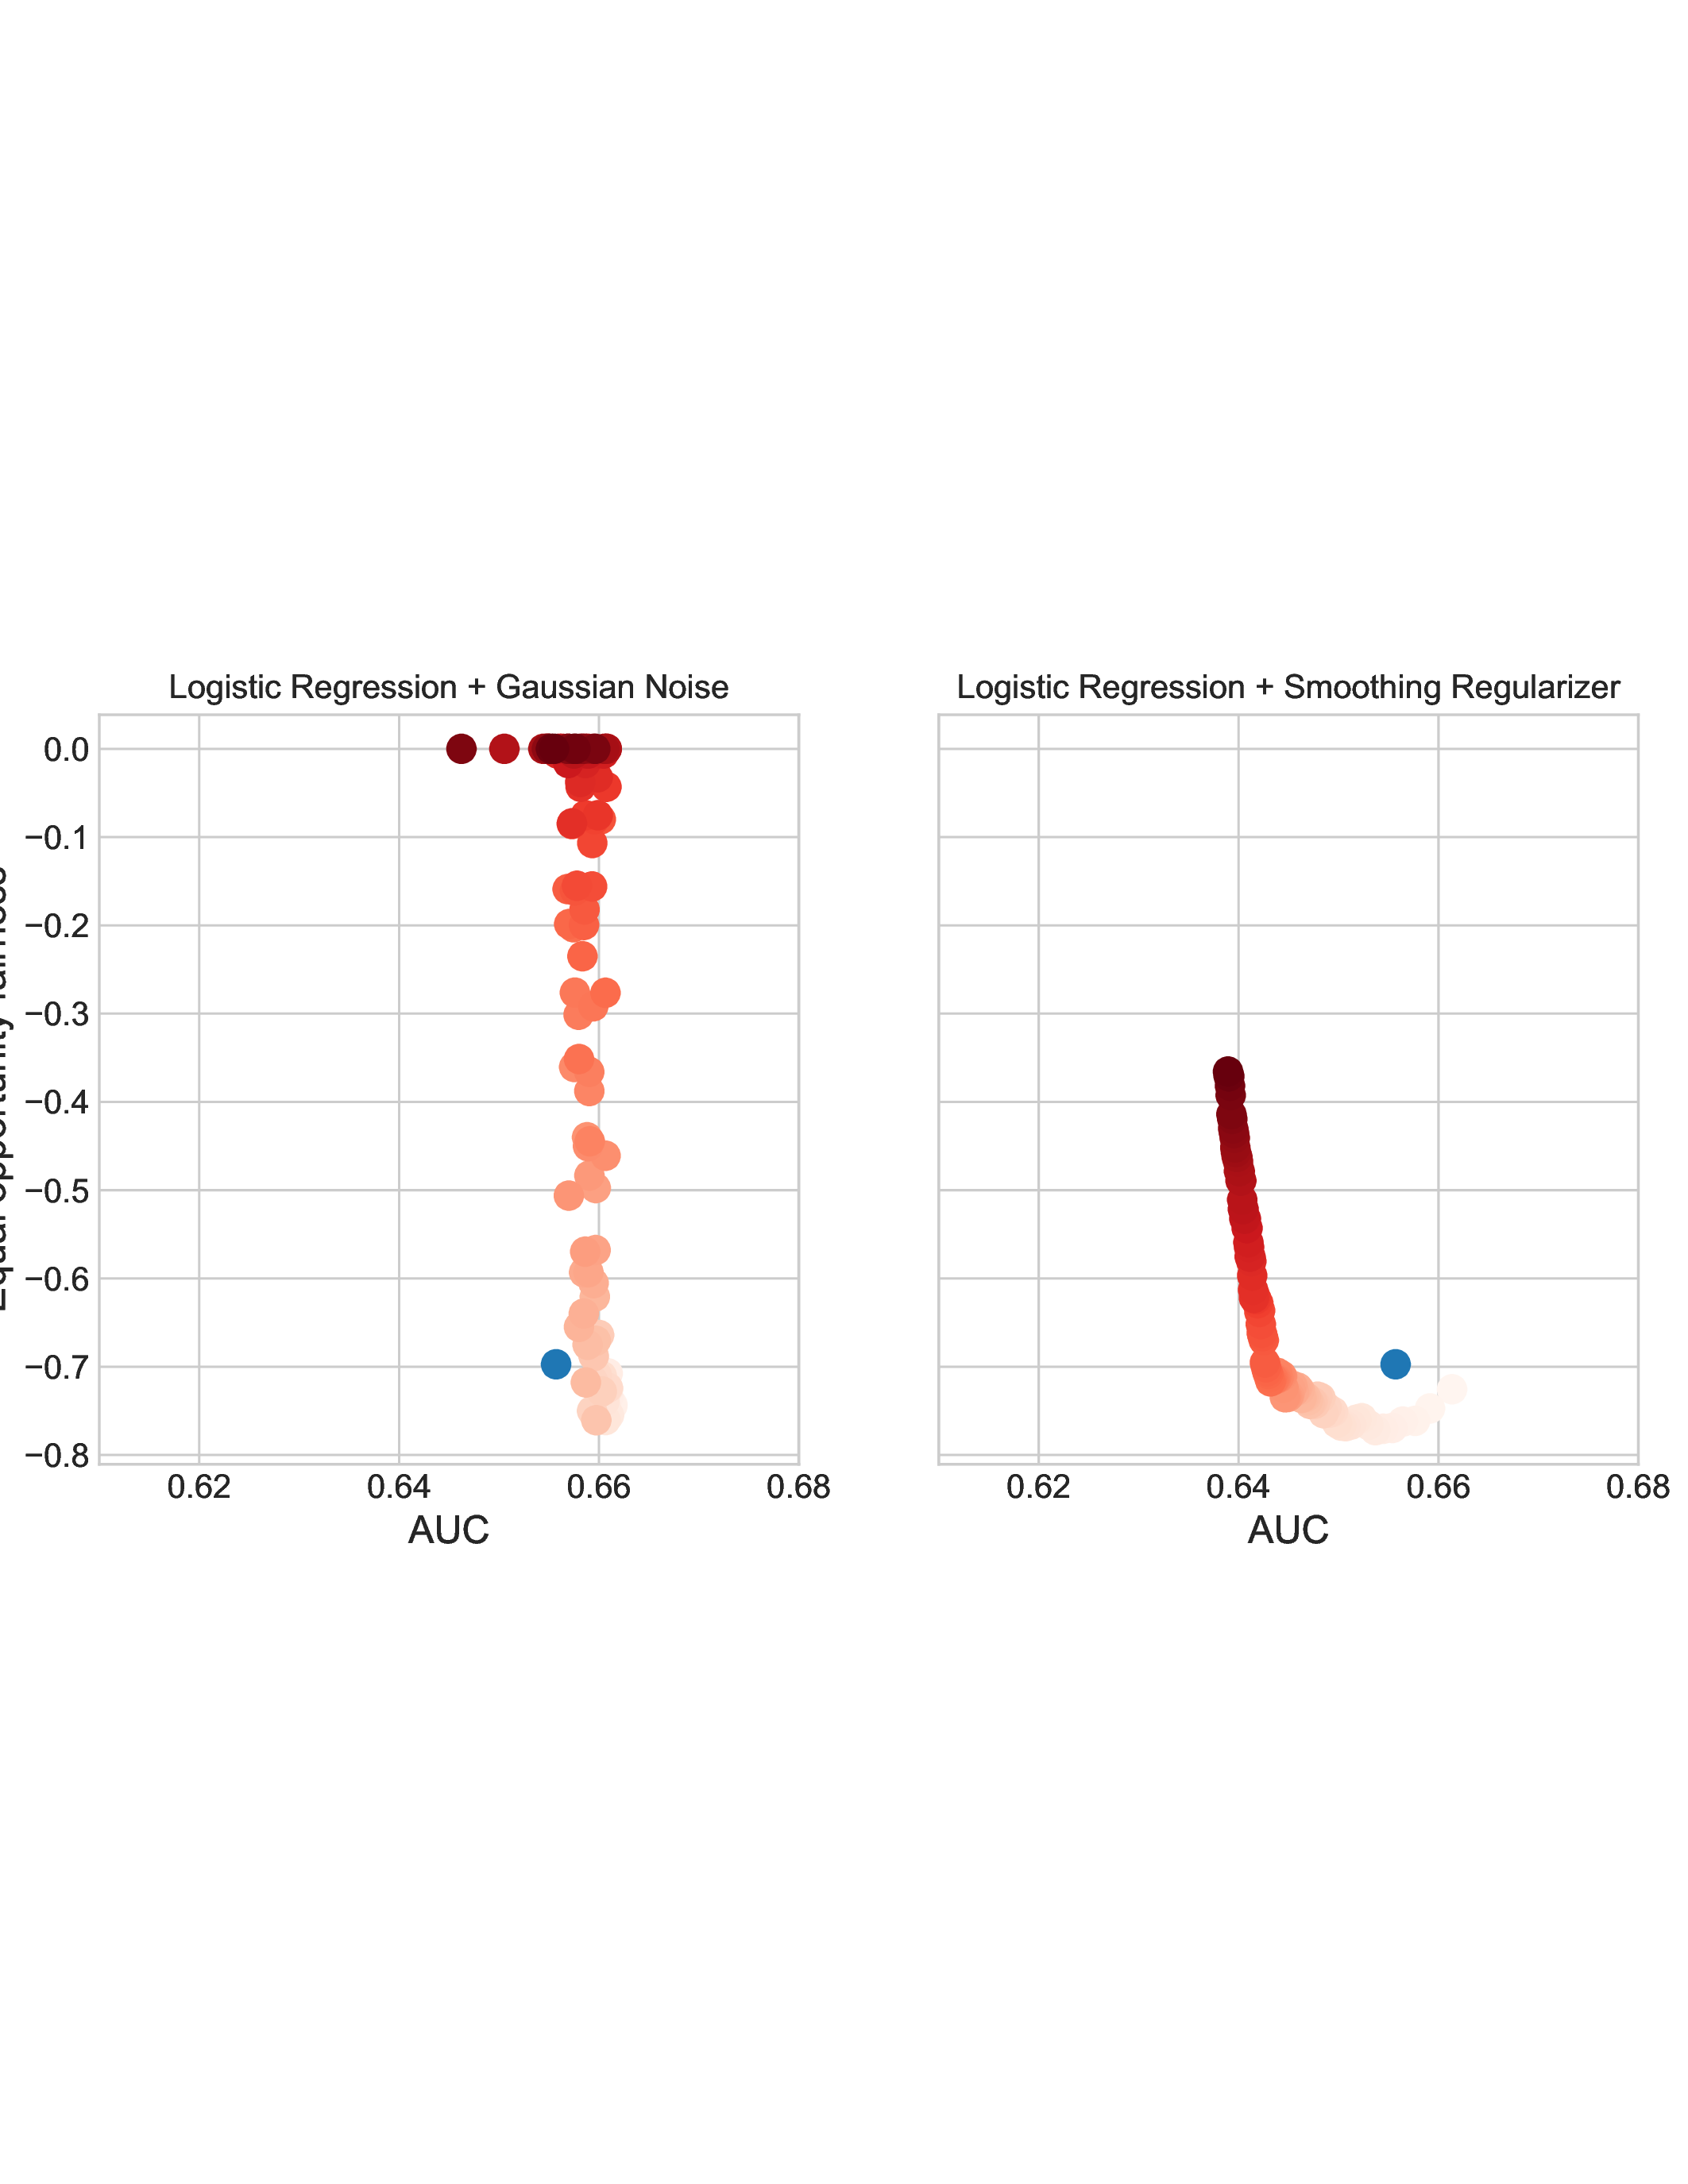}
    \caption{Comparing one-hot encoding and target encoding regularization (Gaussian noise and smoothing) for the Logistic Regression over the test set of the Law School Admission Council survey dataset under intersectional sensitive categorical attributes. Protected group is \textit{BlackFemale}. Reference group is \textit{WhiteMale}. Red dots regard different regularization parameters: the darker the red the higher the regularization. Blue dot regards the one-hot encoding.}
    \label{fig:LawInter}
\end{figure}

In Figure~\ref{fig:LawInter}, we can see how feature concatenation boosts the model performance to an AUC of $0.661$ using one-hot encoding against $0.650$ for the single group case (Figure~\ref{fig:pieLaw}). In the case before, fairness already achieved the worst-case scenario, an equal opportunity difference of one. In this scenario, the best performance model is not one-hot encoding but target encoding. The smoothing regularization presents a more a transition with less variance across the hyperparameter range.
